# Supplementary material for: Prospective Learning: Learning for a Dynamic Future
Source: arXiv:2411.00109 source file (2025-01-30)
Supplement: Supplementary file 1 [file 6_old_appendix.tex]

% !TEX root = ../neurips_2024_final.tex

The autoregressive Transformer is different from the first two architectures since it is trained on sequences of inputs. 
We hence construct many sequences of length $c$ and use the the first $c-1$ samples as input to the Transformer and make it predict the output of the last sample in the sequence.
\[ (z_r)_{r=s-c}^{s-1} := \left((x_{s-C}, y_{s-C}, s-C), \dots, (x_{s-1}, y_{s-1}, s-1), (x_{s}, 0, s)\right) ,\]
to predict the output $y_s$ at time $s$. 
This translates to minimizing the loss function $l_{tr}$ given by
\todo{Rahul: are you saying that the transformer uses a different loss function? this seems problematic to me.}
\[ \hat l_{tr}(f, Z) := \frac{1}{t-C} \sum_{s=C}^{t} \ell(s, f( (z_r)^{s-1}_{s-c}), y_s) \]
where $f$ is a Transformer.

%From the process, we draw $n_{tr}$ training sequences of length $t$. For each such training sequence, we train an instance of the learner and evaluate it over $n_{te}$ testing sequences sampled from the process, starting from $t+1$ to a fixed future horizon $T$. In our experiments, we set $T=500$. Let $f^{(i)}(\cdot, \cdot)$ be the model trained on the $i$-th training sequence and $\left(x_s^{(i, j)}, y_s^{(i, j)}\right)$ be the (input, output) pair at time $s$ of the $j$-th testing sequence with respect to $i$. Then, we estimate the prospective risk using following equation.
%\begin{equation*}
    %\text{prospective risk at time $t$} = \frac{1}{n_{tr}n_{te}(T-t)} \sum_{i=1}^{n_{tr}} \sum_{j=1}^{n_{te}} \sum_{s=t+1}^T \ell \left(y_s^{(i, j)}, f^{(i)}(x_s^{(i, j)}, s) \right)
%\end{equation*}
%\todo{Rahul:please fix this}
%To guarantee an accurate estimate, we set $n_{tr} = 3$ and $n_{te} = 100$ in our experiments.

\paragraph{Prospective Transformers} 
Unlike the previous two architectures, Transformers can handle a sequence of inputs.
In this work, we will use Transformers which use the past $C$ inputs denoted by $(z_s)_{C-t}^{t}$ to make inferences on future data; $C$ is often referred to as the context window of the Transformer.
We consider a concatenation of the input embedding (inputs passed through fully-connected layer) with the time-encoding $\phi(t)$ and pass the concatenation through multiple Transformer blocks. 
Each Transformer block contains an attention layer followed by an MLP with 2 fully-connected layers. Additionally, the Transformer has a residual connection and Layer norm after the attention and MLP blocks.

In the experimental setup above, we have a training sequence $\{(x_s, y_s, s)\}_{s=1}^t$ observed from some process up to a time $t$. Given this finite history of the process and an input at a future time $s > t$, we are required to learn a model that will accurately predict the corresponding outcome at $s$. In other words, we wish to learn the following conditional distribution,
\begin{equation*}
    \mathbb{P}(Y_s  | (x_s, s); (x_1, y_1, 1), \dots, (x_t, y_t, t)), \ \forall s > t
\end{equation*}
Inspired by the similarity this has with the autoregressive objective used in language modeling, we consider training a Transformer model that, given a $c$-length context window comprising of observations $$(x_s, y_s, s), \dots, (x_{s+c}, y_{s+c-1}, s+c-1),$$ predicts the oulcome $y_{s+c}$ at time $s+c$. 
% Note that when $s = r+C$, this is analogous to an Auto-Regressive Transformer. 
% However, we expect the Transformer to learn multi-step temporal dynamics, by forcing it to make predictions at future time steps, in addition to the immediate next one. We refer to it as the Prospective Transformer, which is trained using the algorithm in ~\Cref{alg:prosp-transformer}.

% \begin{algorithm}
% \caption{Training procedure of the prospective transformer}
% \label{alg:prosp-transformer}
% \begin{algorithmic}
% \Require The training sequence $\{(x_r, y_r, r)\}_{r=1}^t$ where each $y_r$ is one-hot encoded with \texttt{num\_classes} equal to the maximum number of classes per task, context length $c$, time-embedding function $\phi(\cdot)$
% \While{not converged}
%     \State $s \sim \text{Uniform}(\{1, \dots, t-c-1 \})$
%     \State $r \sim \text{Uniform}(\{r+c, \dots, t \})$
%     \State $u \gets {\tt Concatenate}([x_{s}, \dots, x_{s+c}, x_r], \ [y_{s}, \dots, y_{s+c}, 0])$
%     \State $u \gets {\tt Concatenate}(u, \ [\phi(s), \dots, \phi(s+c), \phi(r)])$
%     \State $\hat y_s \gets {\tt TransformerEncoder}(u)$
%     \State Take the gradient descent step on the loss between $y_r$ and $\hat y_r$
% \EndWhile
% \end{algorithmic}
% \end{algorithm}

The Transformer encoder is comprised of $N$  encoder layers from the original architecture in~\citet{vaswani2017attention}. We use the following hyperparameters in each encoder layer: model dimension = $256$, feed forward hidden size = $1024$, number of heads = $8$. For synthetic and MNIST experiments, we set $N=2$. When using the transformer for MNIST, we flatten the images to $784$-dimensional vectors. However, for CIFAR-10, we include a 3-layer fully convolutional (FCN) layer before the Transformer encoder to extract a $320$-dimensional feature vector from the $32 \times 32 \times 3$ image. This FCN + Transformer is trained end-to-end. For synthetic and MNIST, we use $N=2$ encoder layers in the architecture, while we set $N=4$ for CIFAR-10.


\begin{figure}[h]
    \centering
    \includegraphics[width=0.4\textwidth]{NeuRIPS_2024/figures/transformer_comparison.pdf}
    \caption{Prospective risk over time for Transformers using the (1) original time-embedding function from~\citet{vaswani2017attention} \textit{(red)}, and (2) proposed time-embedding function comprising of angular frequencies \textit{(blue)}.}
    \label{fig:transformer-comparison}
\end{figure}
